# Supplementary material for: Bound states of skyrmions and merons near the Lifshitz point
Source: arXiv:1703.09173 source file (2017-03-27)
Supplement: Supplementary file 1 [file Suppl_mater.pdf]

# Bound states of skyrmions and merons near the Lifshitz point - Supplemental Material

Y. A. Kharkov,[1] O.P. Sushkov,[1] and M. Mostovoy[2]

[1]*School of Physics, University of New South Wales, Sydney 2052, Australia*

[2]*Zernike Institute for Advanced Materials, University of Groningen, Nijenborgh, Groningen, Netherlands.*

### Appendix A: Phase diagram of the anisotropic square lattice magnet

The phase diagram in the case of an easy-plane anisotropy, $K < 0$, is identical to the phase diagram of the isotropic Heisenberg model ($K = 0$) studied in Ref. [36]. For an easy-axis anisotropy, $K > 0$, the transition between the uniform FM and modulated phases occurs when the energy of the domain wall separating the FM spin-up and spin-down states vanishes. For $J_2 > 2J_3$, the wave vector of the spiral state is $(q, 0)$ or $(0, q)$("1D spiral") and the normal vector to the domain wall has the same direction. The domain wall perpendicular to the $x$ axis with spins in the $xz$ plane is parametrized by the angle $\theta(x)$:

$$S_z(x) = \cos\theta(x), \quad S_x(x) = \sin\theta(x). \tag{A1}$$

The expression for the domain wall energy is obtained by substituting Eq. (??) in Eq. (2):

$$E_{\rm DW} = \frac{L_\perp}{2}\int\limits_{-\infty}^{\infty} dx\left[\rho(\theta')^2 + b_1\left\{(\theta'')^2 + (\theta')^4\right\} + K\sin^2\theta\right], \tag{A2}$$

where $L_\perp$ is the length of the domain wall in the $y$-direction. Using the Ansatz for the domain wall profile,

$$\cos\theta(x) = \tanh\left(\frac{x}{l}\right), \tag{A3}$$

where the domain wall width, $l$, is the variational parameter, we obtain

$$E_{\rm DW}(l) = L_\perp\left[\frac{\rho}{l} + \frac{b_1}{l^3} + Kl\right], \tag{A4}$$

which gives

$$\begin{cases} 3b_1 + \rho l^2 - Kl^4 &= 0, \\ b_1 + \rho l^2 + Kl^4 &= 0, \end{cases} \tag{A5}$$

where the first equation comes from minimization of $E_{\rm DW}(l)$ with respect to $l$ and the second one is $E_{\rm DW} = 0$. The solution of Eq.(??) gives

$$l = \left[\frac{b_1}{K}\right]^{1/4} \tag{A6}$$

and

$$\rho = -2\sqrt{b_1 K}. \tag{A7}$$

Since $b_1 = J_3 - \frac{\rho}{12}$, the critical value of $\rho$ is given by

$$\rho \approx -2\sqrt{J_3 K}. \tag{A8}$$

If the normal to the domain wall makes an angle $\alpha$ with the $x$ axis, then $b_1$ in Eq.(??) is replaced by

$$b_1 + \frac{(b_2 - 2b_1)}{4}\sin^2 2\alpha. \tag{A9}$$

For $J_2 < 2J_3$, the incommensurate state is the "2D spiral" with the wave vector $(q, \pm q)$, corresponding to $\alpha = \pm\frac{\pi}{4}$. In this case, $b_1$ in Eqs.(??) and (??) is replaced by $\frac{2b_1+b_2}{4} \approx \frac{2J_3+J_2}{4}$.

## Appendix B: Details of the numerical procedure

Minimal-energy spin configurations of the model Eq. (1) are found by solving Landau-Lifshitz-Gilbert (LLG) equation with a large damping term on the $51 \times 51$ lattice. The elementary skyrmion configuration for $K > 0$ is obtained starting from the uniform spin-up FM state with a single spin flipped ($S_i^z = -1$) in the center of the lattice and the constraint $S_i^z = -1$ is kept in the initial state of the LLG evolution. To find the bi-meron configuration for $K < 0$, we begin with the elementary skyrmion configuration rotated around the $x$ axis through the angle $\pi/2$: $(S^x, S^y, S^z) \to (S^x, -S^z, S^y)$. Multi-$Q$ skyrmion/meron configurations are obtained by merging $Q$ elementary skyrmions/merons.

The skyrmion-skyrmion interaction potential, $U_{12}(r)$, is found by imposing the constraint $S_z = -1$ in the centers of the two skyrmions separated by the distance $r$. To find the meron-meron interaction potential, we impose constraints $S_z = -1$ and $S_z = 1$ in the centers of the merons.

## Appendix C: Variational description of elementary skyrmions

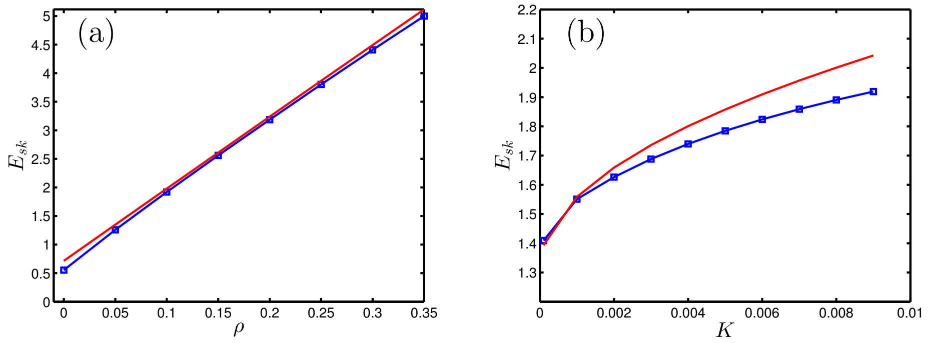


Figure 1: Skyrmion energy versus (a) the spin stiffness, $\rho = J_1 - 2J_2 - 4J_3$, and (b) the strength of the easy-axis anisotropy, $K > 0$, obtained by numerical solution of LLG equation (blue line) and using the variational Ansatz Eq.(**??**). The energy is measured in units of $J_1 = 1$. The model parameters are $J_3 = 0.05$, $K = 5 \cdot 10^{-3}$ (panel a) and $J_2 = 0.45$, $J_3 = 0$ (panel b).

We rewrite Eq. (2) in the form

$$E = \frac{1}{2} \int d^2 r \left[ \rho (\partial_i \boldsymbol{S})^2 + b_1 (\triangle \boldsymbol{S})^2 + (b_2 - 2b_1) \partial_x^2 \boldsymbol{S} \cdot \partial_y^2 \boldsymbol{S} + K(1 - S_z^2) \right], \tag{C1}$$

to separate the spatially isotropic fourth-order term, $b_1(\triangle S_\mu)^2$, from the anisotropic one, $(b_2 - 2b_1)\partial_x^2 \boldsymbol{S} \cdot \partial_y^2 \boldsymbol{S}$. Substituting the Ansatz, $\theta(r) = \pi e^{-r/R}$, for the polar angle $\theta$ describing $\boldsymbol{S}$ into Eq. (**??**), we obtain

$$E = \rho I_\rho + \frac{b_1}{R^2} I_{\text{iso}} + \frac{b_2 - 2b_1}{R^2} I_{\text{ani}} + K R^2 I_K, \tag{C2}$$

where $I_\rho$, $I_{\text{iso}}$, $I_{\text{ani}}$, and $I_K$ are dimensionless integrals that can be calculated numerically:

$$I_K = \frac{\pi}{2} \int_0^\infty dx x \sin^2 \theta(x) \approx 3.96, \quad I_\rho = \pi \int_0^\infty dx x \left[ \frac{1}{x^2} \sin^2(\theta(x)) + (\theta'(x))^2 \right] \approx 13.17,$$

$$I_{\text{iso}} = \pi \int_0^\infty dx x \left[ \left( \Delta_x \sin\theta(x) - \frac{\sin\theta(x)}{x^2} \right)^2 + (\Delta_x \cos\theta(x))^2 \right] \approx 73.87,$$

$$I_{\text{ani}} = \frac{\pi}{8} \int_0^\infty \frac{dx}{x^3} \left[ -3\sin^2\theta(x) + 3x\theta'(x)\sin 2\theta(x) + x^2(\theta'(x))^2(2 - 5\cos 2\theta(x)) + x^4(\theta'(x))^4 - 3x^2(\sin 2\theta(x) - 2x\theta'(x))\theta''(x) + x^4(\theta''(x))^2 \right] \approx 9.23. \tag{C3}$$

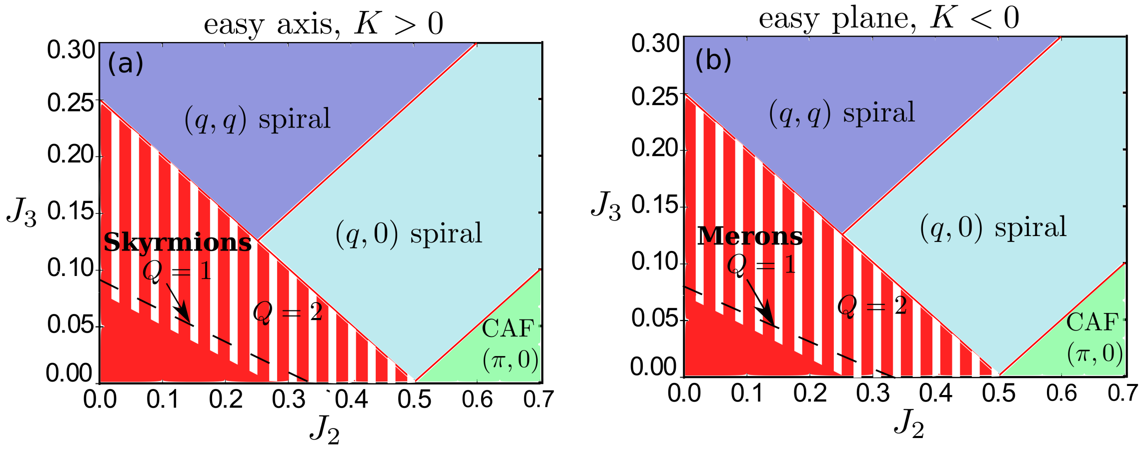


Figure 2: Stability regions of $Q = 2$ skyrmions for $K = -10^{-3}$ (panel a) and bi-merons for $K = -10^{-3}$ indicated by stripes. Dashed lines show the borders of the stability regions of elementary skyrmions and bi-merons with $Q = 1$.

Here, $\theta(x) = \pi e^{-x}$ and $\Delta_x = \partial_{xx} + \frac{1}{x}\partial_x$ is the radial part of the two-dimensional Laplace operator.

The variational energy Eq. (**??**) has a minimum at the optimal skyrmion radius,

$$R = \left( \frac{b_1 I_{\text{iso}} + (b_2 - 2b_1) I_{\text{ani}}}{K I_K} \right)^{1/4}. \tag{C4}$$

The skyrmion radius $R \gg 1$, for $0 < K \ll 1$. The variational energy of the elementary skyrmion with $|Q| = 1$ is

$$E_{Q=\pm 1} = \rho I_\rho + 2\sqrt{(b_1 I_{\text{iso}} + (b_2 - 2b_1) I_{\text{ani}}) K I_K}. \tag{C5}$$

For $b_1 = b_2 = K = 0$, Eq. (**??**) can be compared with the energy $4\pi\rho$ of the Belavin-Polyakov skyrmion with $Q = \pm 1$ in the $O(3)$ nonlinear sigma model. Our variational result, $\sim 13.17\rho$, is larger by 5%.

### Appendix D: Variational description of meron pairs

The variational description of meron pairs with the isotropic topological density profile, i.e. bi-merons shown in Figs. 5 (b,e) with a "round" distribution of the topological charge density, can be developed by analogy with the variational treatment of skyrmions. The simplest "isotropic" parametrization for the meron pair reads, $\boldsymbol{S} = (\sin\theta(r)\cos\phi, -\cos\theta(r)\sin(\phi+\chi), \sin\theta(r)\sin(\phi+\chi))$, where $\chi$ is the helicity angle and $\theta(r) = \pi e^{-r/R}$. Since the first three terms in Eq.(**??**) describing the exchange energy are invariant under global rotations in the spin space, the integrals $I_\rho$, $I_{\text{iso}}$ and $I_{\text{ani}}$ are independent of the sign of $K$. For an easy-plane anisotropy $K < 0$, the magnetic anisotropy term in energy is $-K/2\int d^2r S_z^2(r) = -\pi K/2 \int dr r \sin^2\theta(r) = |K| I_K R^2$ (see Eqs. (**??**) and (**??**)). Therefore, the variational energy and characteristic size of the meron pair remain the same as for the skyrmion (see Eqs. (**??**) and (**??**)) provided that $K$ is replaced with $|K|$. This variational treatment of bi-merons disregards any effects of spatial anisotropy and, therefore, cannot describe meron fractionalization.

### Appendix E: Stability of skyrmions and bi-merons with higher $Q$

Attraction between topological defects for $\rho > 0$ lowers the energy of the multi-$Q$ skyrmions and bi-merons making them more stable than the elementary skyrmions and bi-merons. Figure 2 shows stability regions in the $J_2 - J_3$ phase diagram for the $|Q| = 2$ and $|Q| = 1$ skyrmions (panel a) and bi-merons (panel b). The stability regions of multi-$Q$ skyrmions increases with $|Q|$.
